# Supplementary material for: PlaySlot: Learning Inverse Latent Dynamics for Controllable Object-Centric Video Prediction and Planning
Source: arXiv:2502.07600 source file (2025-05-21)
Supplement: Supplementary file 1 [file button_00.tex]

\resizebox{1.0 \linewidth}{!}{
		\begin{tikzpicture} 
			%
			% SIMULATION
			%
			\node(sim_0)[anchor=north, inner sep=0, outer sep=0] at (0,0.0) 
			{\includegraphics[height=3cm]
				{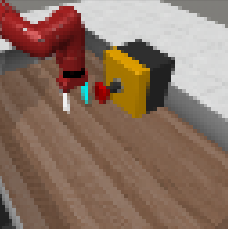}
			};
			\draw[black](sim_0.south west) rectangle (sim_0.north east);
			%
			%
			%
			%
			% LATENT IMAGINATION
			%
			%
			\node(pred_1)[anchor=west, inner sep=0, outer sep=0] at ([xshift=1.0cm, yshift=0cm]sim_0.north east) 
			{\includegraphics[height=3cm]
				{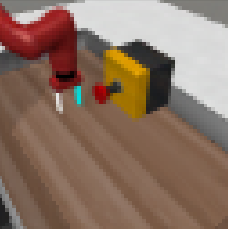}
			};
			\draw[black](pred_1.south west) rectangle (pred_1.north east);
			\node(pred_3)[anchor=west, inner sep=0, outer sep=0] at ([xshift=0.00cm]pred_1.east) 
			{\includegraphics[height=3cm]
				{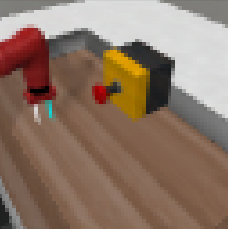}
			};
			\draw[black](pred_3.south west) rectangle (pred_3.north east);
			\node(pred_5)[anchor=west, inner sep=0, outer sep=0] at ([xshift=0.00cm]pred_3.east) 
			{\includegraphics[height=3cm]
				{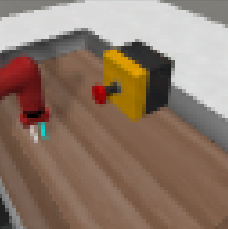}
			};
			\draw[black](pred_5.south west) rectangle (pred_5.north east);
			\node(pred_7)[anchor=west, inner sep=0, outer sep=0] at ([xshift=0.00cm]pred_5.east) 
			{\includegraphics[height=3cm]
				{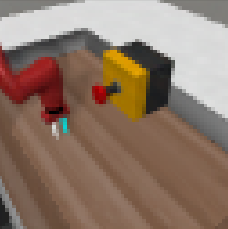}
			};
			\draw[black](pred_7.south west) rectangle (pred_7.north east);
			\node(pred_9)[anchor=west, inner sep=0, outer sep=0] at ([xshift=0.00cm]pred_7.east) 
			{\includegraphics[height=3cm]
				{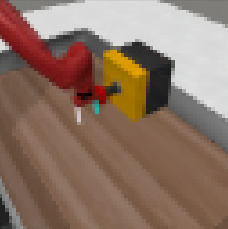}
			};
			\draw[black](pred_9.south west) rectangle (pred_9.north east);
			\node(pred_11)[anchor=west, inner sep=0, outer sep=0] at ([xshift=0.00cm]pred_9.east) 
			{\includegraphics[height=3cm]
				{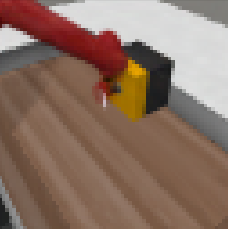}
			};
			\draw[black](pred_11.south west) rectangle (pred_11.north east);
			\node(0)[anchor=south,draw=none,ultra thick,inner sep=0, outer sep=0] at
			([xshift=-0.3cm, yshift=-1.55cm]pred_1.west)
			{\large{\rotatebox{90}{\textbf{Latent Behavior}}}};
			\node(sim_1)[anchor=north, inner sep=0, outer sep=0] at ([xshift=0.00cm]pred_1.south) 
			{\includegraphics[height=3cm]
				{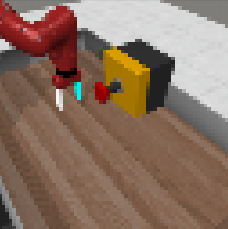}
			};
			\draw[black](sim_1.south west) rectangle (sim_1.north east);
			\node(sim_3)[anchor=west, inner sep=0, outer sep=0] at ([xshift=0.00cm]sim_1.east) 
			{\includegraphics[height=3cm]
				{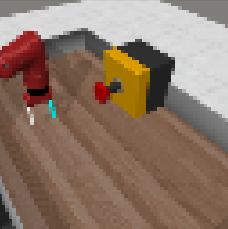}
			};
			\draw[black](sim_3.south west) rectangle (sim_3.north east);
			\node(sim_5)[anchor=west, inner sep=0, outer sep=0] at ([xshift=0.00cm]sim_3.east) 
			{\includegraphics[height=3cm]
				{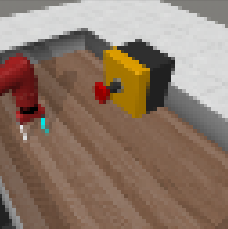}
			};
			\draw[black](sim_5.south west) rectangle (sim_5.north east);
			\node(sim_7)[anchor=west, inner sep=0, outer sep=0] at ([xshift=0.00cm]sim_5.east) 
			{\includegraphics[height=3cm]
				{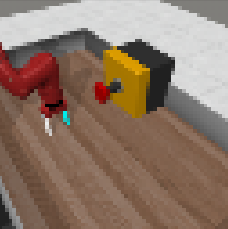}
			};
			\draw[black](sim_7.south west) rectangle (sim_7.north east);
			\node(sim_9)[anchor=west, inner sep=0, outer sep=0] at ([xshift=0.00cm]sim_7.east) 
			{\includegraphics[height=3cm]
				{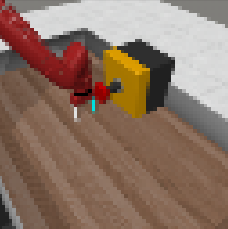}
			};
			\draw[black](sim_9.south west) rectangle (sim_9.north east);
			\node(sim_11)[anchor=west, inner sep=0, outer sep=0] at ([xshift=0.00cm]sim_9.east) 
			{\includegraphics[height=3cm]
				{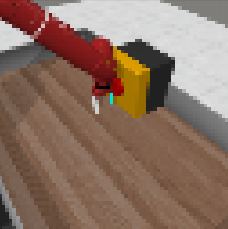}
			};
			\draw[black](sim_11.south west) rectangle (sim_11.north east);
			\node(0)[anchor=south,draw=none,ultra thick,inner sep=0, outer sep=0] at
			([xshift=-0.3cm, yshift=-1.15cm]sim_1.west)
			{\large{\rotatebox{90}{\textbf{Sim. Actions}}}};
			%
			%
			%
			% TIME LABELS
			\node(0)[anchor=south,draw=none,ultra thick,inner sep=0, outer sep=0] at([yshift=0.1cm]sim_0.north)
			{\large{$t=1$}};
			\node(0)[anchor=south,draw=none,ultra thick,inner sep=0, outer sep=0] at([yshift=0.1cm]pred_1.north)
			{\large{$2$}};
			\node(0)[anchor=south,draw=none,ultra thick,inner sep=0, outer sep=0] at([yshift=0.1cm]pred_3.north)
			{\large{$4$}};
			\node(0)[anchor=south,draw=none,ultra thick,inner sep=0, outer sep=0] at([yshift=0.1cm]pred_5.north)
			{\large{$7$}};
			\node(0)[anchor=south,draw=none,ultra thick,inner sep=0, outer sep=0] at([yshift=0.1cm]pred_7.north)
			{\large{$10$}};
			\node(0)[anchor=south,draw=none,ultra thick,inner sep=0, outer sep=0] at([yshift=0.1cm]pred_9.north)
			{\large{$13$}};
			\node(0)[anchor=south,draw=none,ultra thick,inner sep=0, outer sep=0] at([yshift=0.1cm]pred_11.north)
			{\large{$16$}};
			\node(0)[anchor=north,draw=none,ultra thick,inner sep=0, outer sep=0]
			at([xshift=0.0cm, yshift=-0.6cm]sim_0.south)
			{\LARGE a)};
		\end{tikzpicture}
	}
