# Supplementary material for: PlaySlot: Learning Inverse Latent Dynamics for Controllable Object-Centric Video Prediction and Planning
Source: arXiv:2502.07600 source file (2025-05-21)
Supplement: Supplementary file 4 [file fig_quant_beh.tex]

\begin{figure}[t]
	\vspace{0.0cm}
	\hspace{-0.3cm}
	\resizebox{1.0 \linewidth}{!}{
	\begin{tikzpicture} 
		\node(P0)[fill=none] {};
		\node(fig1)[anchor=north west] at (P0) 
		{\includegraphics[height=4cm]{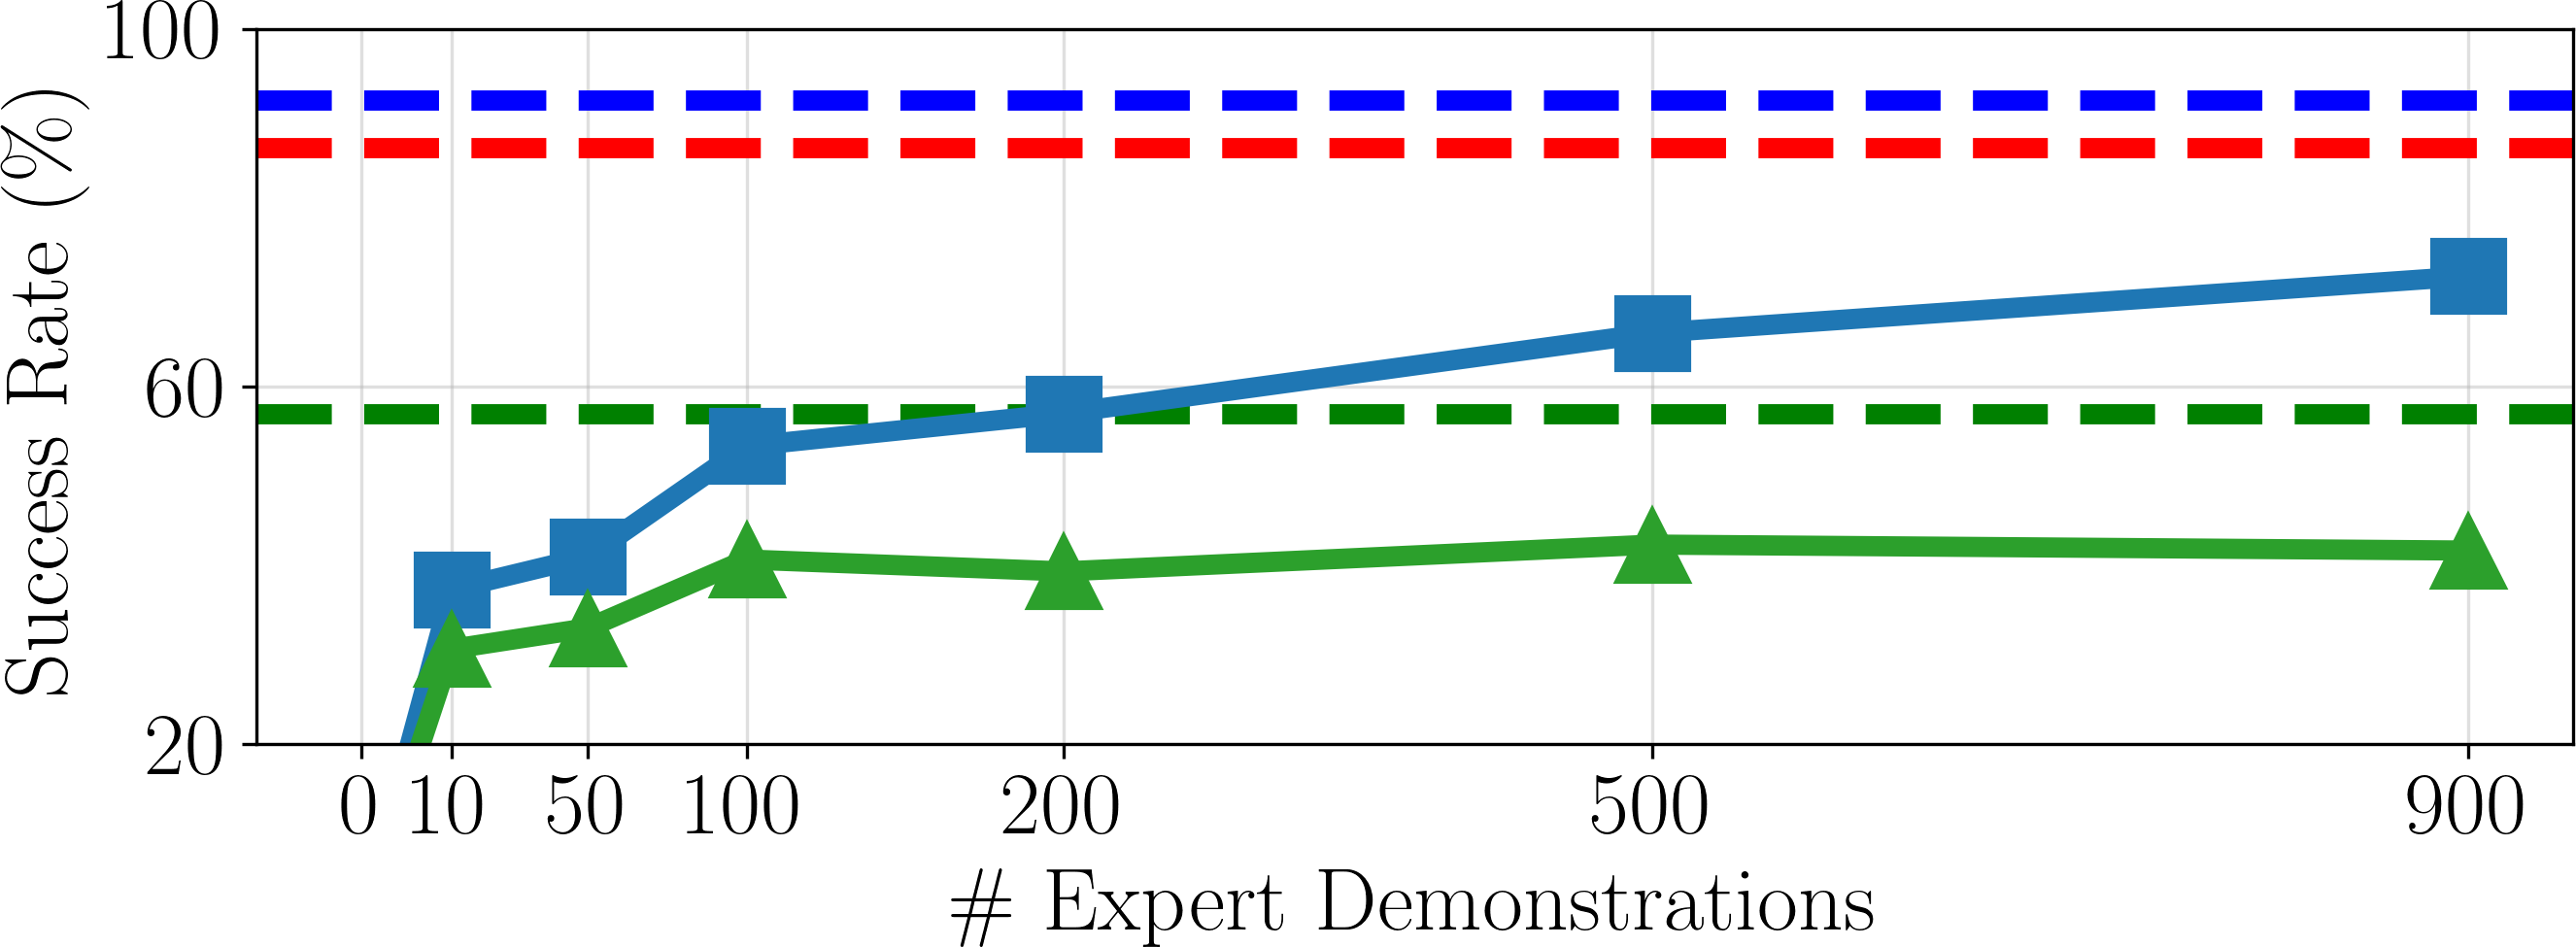}};
		\node(leg1)[anchor=north] at ([xshift=0.4cm, yshift=0cm]fig1.south) 
		{\includegraphics[width=0.58 \linewidth]{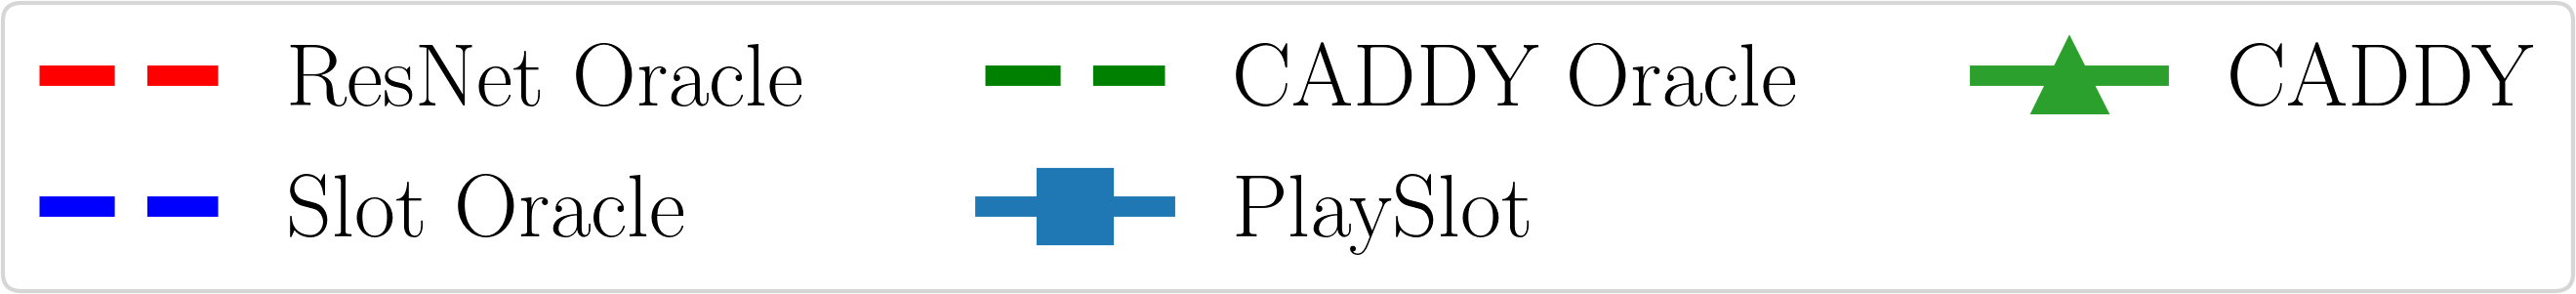}};
		\node(fig2)[anchor=west] at ([xshift=0.2cm, yshift=0cm]fig1.east) 
		{\includegraphics[height=4cm]{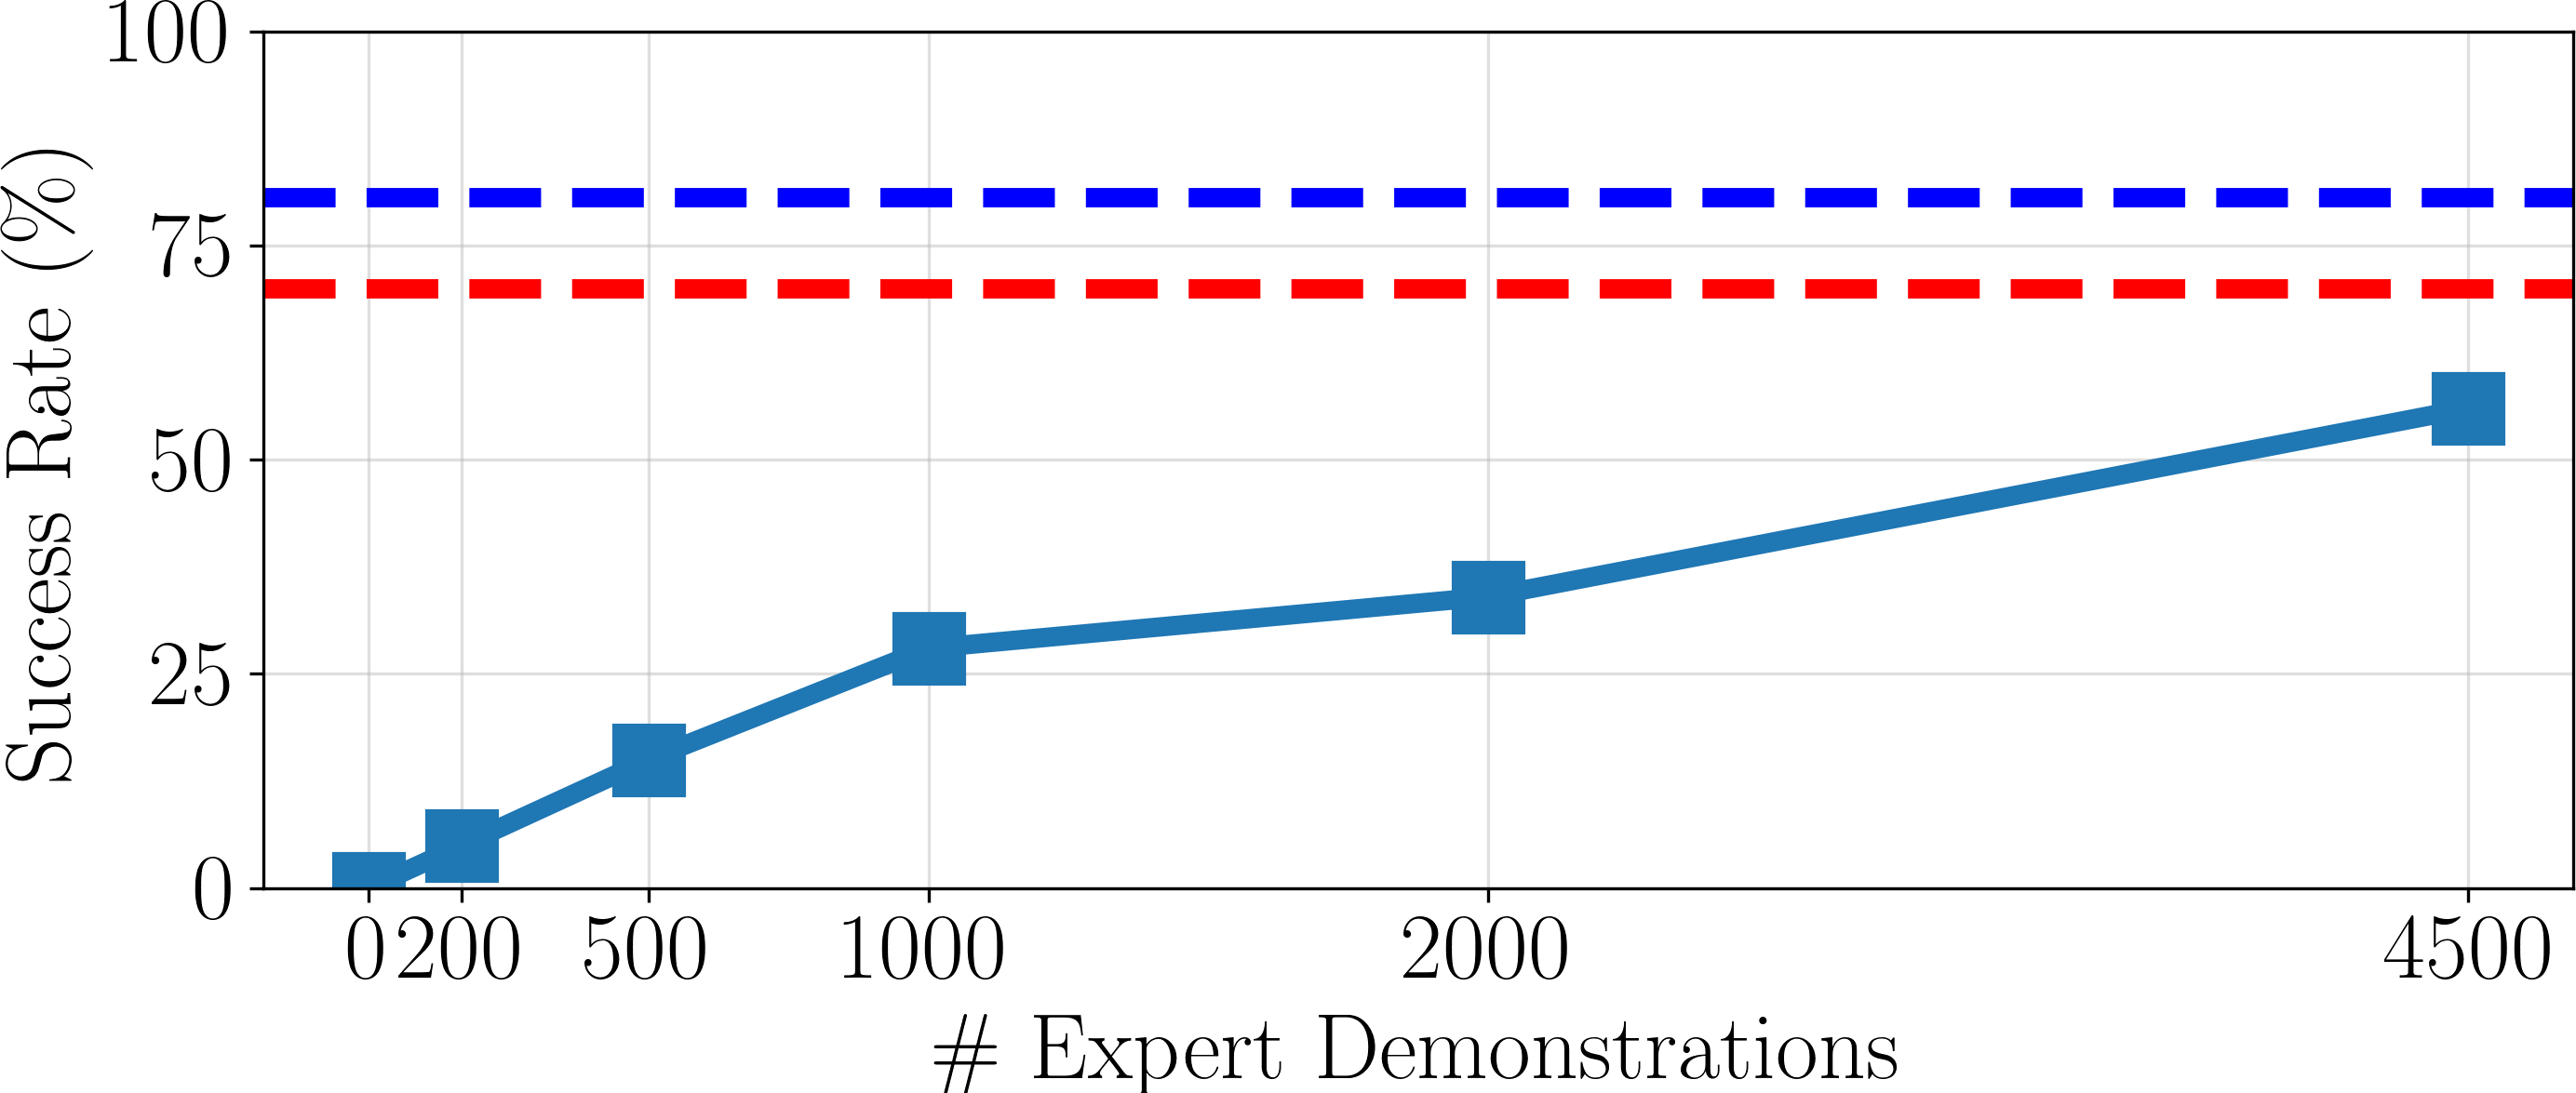}};
		\node(leg2)[anchor=north] at  ([xshift=0.4cm, yshift=0cm]fig2.south) 
		{\includegraphics[width=0.48\linewidth]{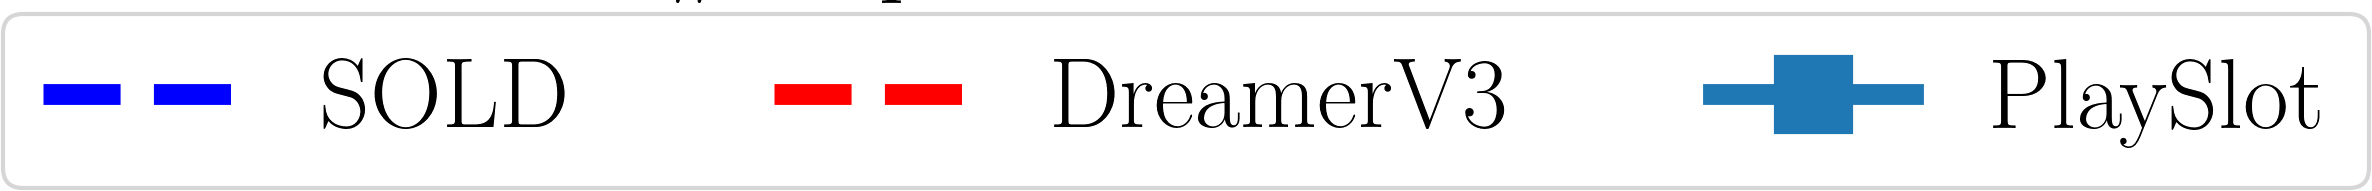}};
		\node(a)[anchor=south] at ([xshift=0.5cm, yshift=-0.2cm]fig1.north) 
		{\large \ButtonPress~Behavior};
		\node(a)[anchor=south] at ([xshift=0.5cm, yshift=-0.2cm]fig2.north) 
		{\large \RobotDB~Behavior};
		\node(a)[anchor=east] at ([xshift=-0.2cm, yshift=0.54cm]leg1.south west) 
		{\Large a)};
		\node(b)[anchor=east] at ([xshift=-0.2cm, yshift=0cm]leg2.south west) 
		{\Large b)};
	\end{tikzpicture}
	}
	\vspace{-0.2cm}
	\caption{
		Success rate (\%) as a function of the number of expert demonstrations for different models on the a) \ButtonPress~and b) \RobotDB~environments.
		Object-centric models (Slot Oracle, \Method~and SOLD) outperform their non-object centric counterparts.
		\Method~consistently improves with more expert demonstrations, outperforming CADDY.		
	}
	\vspace{-0.2cm}
	\label{fig: quant beh}
\end{figure}
