# Supplementary material for: PlaySlot: Learning Inverse Latent Dynamics for Controllable Object-Centric Video Prediction and Planning
Source: arXiv:2502.07600 source file (2025-05-21)
Supplement: Supplementary file 8 [file qual_00.tex]

\resizebox{1.0 \linewidth}{!}{
	\begin{tikzpicture} 
		\node(P0)[fill=none] {};
		%
		%
		% SEED TARGE
		\node(seed)[anchor=north west, inner sep=0, outer sep=0] at (P0) 
		{\includegraphics[height=3cm]
			{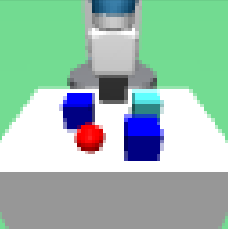}
		};
		\draw[black](seed.south west) rectangle (seed.north east);
		\node(0)[anchor=south,draw=none,ultra thick,inner sep=0, outer sep=0] at
		([xshift=-0.25cm, yshift=-1.65cm]seed.north west)
		{{\rotatebox{90}{\Large GT}}};
		\node(target_00)[anchor=west, inner sep=0, outer sep=0] at
		([xshift=0.00cm]seed.east) 
		{\includegraphics[height=3cm]
			{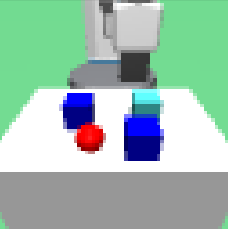}
		};
		\draw[black](target_00.south west) rectangle (target_00.north east);
		\node(target_01)[anchor=west, inner sep=0, outer sep=0] at
		([xshift=0.00cm]target_00.east) 
		{\includegraphics[height=3cm]
			{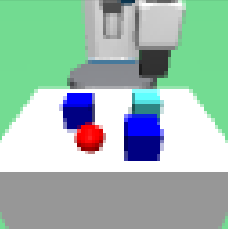}
		};
		\draw[black](target_01.south west) rectangle (target_01.north east);
		\node(target_02)[anchor=west, inner sep=0, outer sep=0] at
		([xshift=0.00cm]target_01.east) 
		{\includegraphics[height=3cm]
			{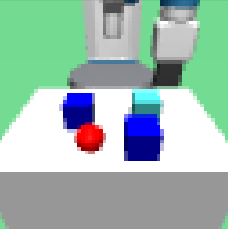}
		};
		\draw[black](target_02.south west) rectangle (target_02.north east);
		\node(target_04)[anchor=west, inner sep=0, outer sep=0] at
		([xshift=0.00cm]target_02.east)
		{\includegraphics[height=3cm]
			{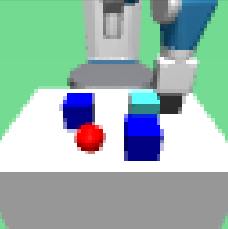}
		};
		\draw[black](target_04.south west) rectangle (target_04.north east);
		\node(target_07)[anchor=west, inner sep=0, outer sep=0] at
		([xshift=0.00cm]target_04.east)
		{\includegraphics[height=3cm]
			{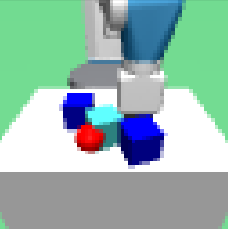}
		};
		\draw[black](target_07.south west) rectangle (target_07.north east);
		\node(target_11)[anchor=west, inner sep=0, outer sep=0] at
		([xshift=0.00cm]target_07.east)
		{\includegraphics[height=3cm]
			{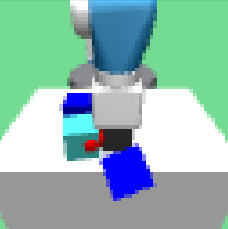}
		};
		\draw[black](target_11.south west) rectangle (target_11.north east);
		\node(target_14)[anchor=west, inner sep=0, outer sep=0] at
		([xshift=0.00cm]target_11.east)
		{\includegraphics[height=3cm]
			{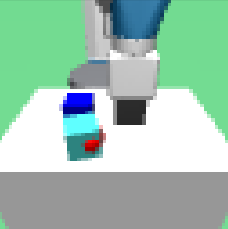}
		};
		\draw[black](target_14.south west) rectangle (target_14.north east);
		%
		%
		%
		% PLAYSLOT
		\node(playslot_00)[anchor=north, inner sep=0, outer sep=0] at
		([xshift=0.00cm]target_00.south) 
		{\includegraphics[height=3cm]
			{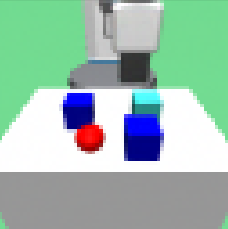}
		};
		\draw[black](playslot_00.south west) rectangle (playslot_00.north east);
		\node(playslot_01)[anchor=north, inner sep=0, outer sep=0] at
		([xshift=0.00cm]target_01.south) 
		{\includegraphics[height=3cm]
			{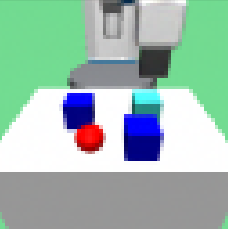}
		};
		\draw[black](playslot_01.south west) rectangle (playslot_01.north east);
		\node(playslot_02)[anchor=north, inner sep=0, outer sep=0] at
		([xshift=0.00cm]target_02.south) 
		{\includegraphics[height=3cm]
			{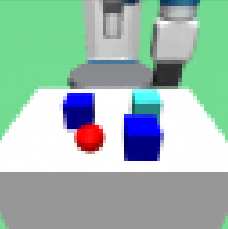}
		};
		\draw[black](playslot_02.south west) rectangle (playslot_02.north east);
		\node(playslot_04)[anchor=north, inner sep=0, outer sep=0] at
		([xshift=0.00cm]target_04.south) 
		{\includegraphics[height=3cm]
			{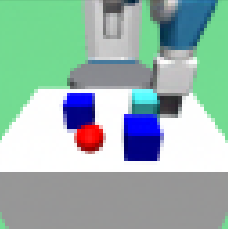}
		};
		\draw[black](playslot_04.south west) rectangle (playslot_04.north east);
		\node(playslot_07)[anchor=north, inner sep=0, outer sep=0] at
		([xshift=0.00cm]target_07.south) 
		{\includegraphics[height=3cm]
			{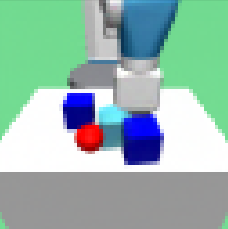}
		};
		\draw[black](playslot_07.south west) rectangle (playslot_07.north east);
		\node(playslot_11)[anchor=north, inner sep=0, outer sep=0] at
		([xshift=0.00cm]target_11.south) 
		{\includegraphics[height=3cm]
			{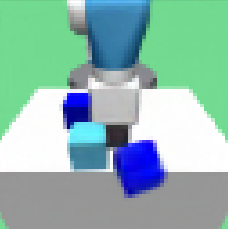}
		};
		\draw[black](playslot_11.south west) rectangle (playslot_11.north east);
		\node(playslot_14)[anchor=north, inner sep=0, outer sep=0] at
		([xshift=0.00cm]target_14.south) 
		{\includegraphics[height=3cm]
			{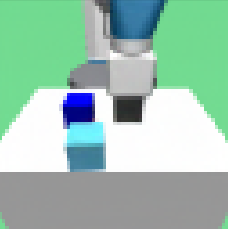}
		};
		\draw[black](playslot_14.south west) rectangle (playslot_14.north east);
		\node(PlaySlotLabel)[anchor=east,draw=none,ultra thick,inner sep=0, outer sep=0] at 	([xshift=-0.5cm, yshift=0.0cm]playslot_00.west)
		{\Large{\Method}};
		%
		%
		%
		%
		% SVG
		\node(svg_00)[anchor=north, inner sep=0, outer sep=0] at
		([xshift=0.00cm]playslot_00.south) 
		{\includegraphics[height=3cm]
			{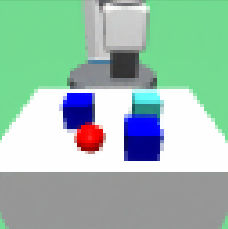}
		};
		\draw[black](svg_00.south west) rectangle (svg_00.north east);
		\node(svg_01)[anchor=north, inner sep=0, outer sep=0] at
		([xshift=0.00cm]playslot_01.south) 
		{\includegraphics[height=3cm]
			{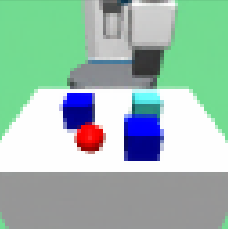}
		};
		\draw[black](svg_01.south west) rectangle (svg_01.north east);
		\node(svg_02)[anchor=north, inner sep=0, outer sep=0] at
		([xshift=0.00cm]playslot_02.south) 
		{\includegraphics[height=3cm]
			{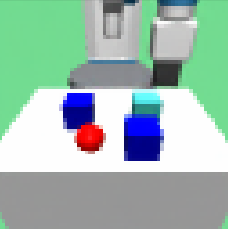}
		};
		\draw[black](svg_02.south west) rectangle (svg_02.north east);
		\node(svg_04)[anchor=north, inner sep=0, outer sep=0] at
		([xshift=0.00cm]playslot_04.south) 
		{\includegraphics[height=3cm]
			{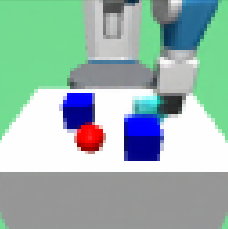}
		};
		\draw[black](svg_04.south west) rectangle (svg_04.north east);
		\node(svg_07)[anchor=north, inner sep=0, outer sep=0] at
		([xshift=0.00cm]playslot_07.south) 
		{\includegraphics[height=3cm]
			{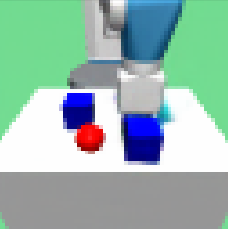}
		};
		\draw[black](svg_07.south west) rectangle (svg_07.north east);
		\node(svg_11)[anchor=north, inner sep=0, outer sep=0] at
		([xshift=0.00cm]playslot_11.south) 
		{\includegraphics[height=3cm]
			{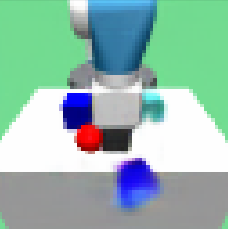}
		};
		\draw[black](svg_11.south west) rectangle (svg_11.north east);
		\node(svg_14)[anchor=north, inner sep=0, outer sep=0] at
		([xshift=0.00cm]playslot_14.south) 
		{\includegraphics[height=3cm]
			{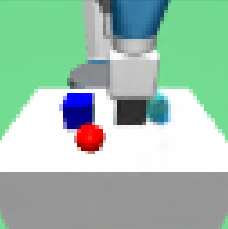}
		};
		\draw[black](svg_14.south west) rectangle (svg_14.north east);
		\node(PlaySlotLabel)[anchor=east,draw=none,ultra thick,inner sep=0, outer sep=0] at 	([xshift=-0.5cm, yshift=0.0cm]svg_00.west)
		{\Large{SVG}};
		%
		%
		%
		% SVG
		\node(CADDY_00)[anchor=north, inner sep=0, outer sep=0] at
		([xshift=0.00cm]svg_00.south) 
		{\includegraphics[height=3cm]
			{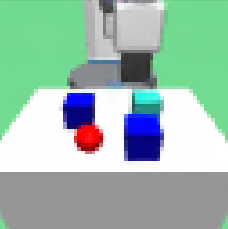}
		};
		\draw[black](CADDY_00.south west) rectangle (CADDY_00.north east);
		\node(CADDY_01)[anchor=north, inner sep=0, outer sep=0] at
		([xshift=0.00cm]svg_01.south) 
		{\includegraphics[height=3cm]
			{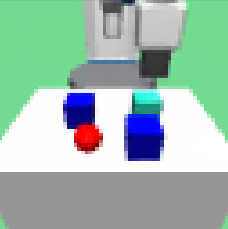}
		};
		\draw[black](CADDY_01.south west) rectangle (CADDY_01.north east);
		\node(CADDY_02)[anchor=north, inner sep=0, outer sep=0] at
		([xshift=0.00cm]svg_02.south) 
		{\includegraphics[height=3cm]
			{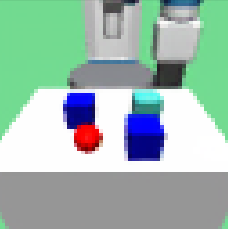}
		};
		\draw[black](CADDY_02.south west) rectangle (CADDY_02.north east);
		\node(CADDY_04)[anchor=north, inner sep=0, outer sep=0] at
		([xshift=0.00cm]svg_04.south) 
		{\includegraphics[height=3cm]
			{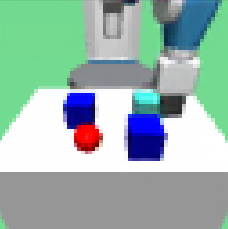}
		};
		\draw[black](CADDY_04.south west) rectangle (CADDY_04.north east);
		\node(CADDY_07)[anchor=north, inner sep=0, outer sep=0] at
		([xshift=0.00cm]svg_07.south) 
		{\includegraphics[height=3cm]
			{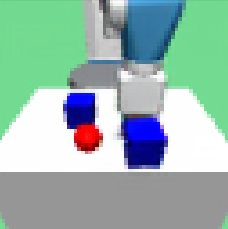}
		};
		\draw[black](CADDY_07.south west) rectangle (CADDY_07.north east);
		\node(CADDY_11)[anchor=north, inner sep=0, outer sep=0] at
		([xshift=0.00cm]svg_11.south) 
		{\includegraphics[height=3cm]
			{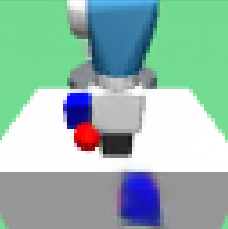}
		};
		\draw[black](CADDY_11.south west) rectangle (CADDY_11.north east);
		\node(CADDY_14)[anchor=north, inner sep=0, outer sep=0] at
		([xshift=0.00cm]svg_14.south) 
		{\includegraphics[height=3cm]
			{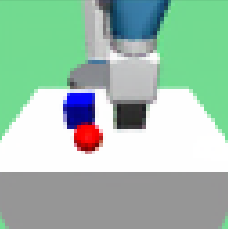}
		};
		\draw[black](CADDY_14.south west) rectangle (CADDY_14.north east);
		\node(PlaySlotLabel)[anchor=east,draw=none,ultra thick,inner sep=0, outer sep=0] at 	([xshift=-0.5cm, yshift=0.0cm]CADDY_00.west)
		{\Large{CADDY}};
		%
		%
		%
		%
		% TIME LABELS
		\node(0)[anchor=south,draw=none,ultra thick,inner sep=0, outer sep=0] at 	([yshift=0.1cm]seed.north)
		{\large{$t=0$}};
		\node(0)[anchor=south,draw=none,ultra thick,inner sep=0, outer sep=0] at 	([yshift=0.1cm]target_00.north)
		{\large{$1$}};
		\node(0)[anchor=south,draw=none,ultra thick,inner sep=0, outer sep=0] at 	([yshift=0.1cm]target_01.north)
		{\large{$2$}};
		\node(0)[anchor=south,draw=none,ultra thick,inner sep=0, outer sep=0] at 	([yshift=0.1cm]target_02.north)
		{\large{$3$}};
		\node(0)[anchor=south,draw=none,ultra thick,inner sep=0, outer sep=0] at 	([yshift=0.1cm]target_04.north)
		{\large{$5$}};
		\node(0)[anchor=south,draw=none,ultra thick,inner sep=0, outer sep=0] at 	([yshift=0.1cm]target_07.north)
		{\large{$8$}};
		\node(0)[anchor=south,draw=none,ultra thick,inner sep=0, outer sep=0] at 	([yshift=0.1cm]target_11.north)
		{\large{$12$}};
		\node(0)[anchor=south,draw=none,ultra thick,inner sep=0, outer sep=0] at 	([yshift=0.1cm]target_14.north)
		{\large{$15$}};
		\node(0)[anchor=north,draw=none,ultra thick,inner sep=0, outer sep=0] at 
		([xshift=-0.7cm, yshift=-0.7cm]PlaySlotLabel.south)
		{\LARGE{a)}};
	\end{tikzpicture}
}
